# Supplementary material for: Efficient molecular quantum dynamics in coordinate and phase space using pruned bases
Source: arXiv:1606.04004 ancillary file (2016-11-15)
Supplement: Supplementary file 1 [file esi_pWeylet.pdf]

# *Supplementary information for* **Efficient molecular quantum dynamics in coordinate and phase space using pruned bases**

H. R. Larsson[1] B. Hartke[1] D. J. Tannor[2]

[1]Institut für Physikalische Chemie, Christian-Albrechts-Universität zu Kiel, 24098 Kiel, Germany
[2] Department of Chemical Physics, Weizmann Institute of Science, 76100 Rehovot, Israel

Journal of Chemical Physics

## i. Comparison of the basis transformations

For the transformation of the matrix elements from the momentum-symmetrized Gaussian to the Weylet basis, we closely follow Ref. 1. The Weylet functions $\langle x \,|\, \overline{w} \rangle$ are given by a linear combination of momentum-symmetrized Gaussians,

$$|\overline{w}_{st}\rangle = \sum_{m=-m_{\max}}^{m_{\max}} \sum_{n=-m_{\max}}^{m_{\max}} (-1)^{n/2+mt} S_{mn}^{-1/2} \left|\widetilde{\phi}_{uv}\right\rangle , \tag{i}$$

where $u = s + m, v = t + n$ and $t$ is half-integer.[1] $\langle x| \widetilde{\phi}_{uv}\rangle$ are given in Eq. (20) in the main article. The summation is only over even position and momentum indices, $m$ and $n$.[2] Further, one can apply a "symplicial" truncation using the restriction $|m| + |n| \leq m_{\max}$.[3] $m_{\max}$ is chosen to be 10 which is the value used in Table 1 in Ref. 2. If lower accuracy is sufficient, smaller values can be used.

One transformed matrix element is then evaluated as

$${}^{\overline{w}}H_{sts't'} = \sum_{m=-m_{\max}}^{m_{\max}} \sum_{n=-m_{\max}}^{m_{\max}} \sum_{m'=-m_{\max}}^{m_{\max}} \sum_{n'=-m_{\max}}^{m_{\max}} (-1)^{n/2+mt+n'/2+m't'} S_{mn}^{-1/2} S_{m'n'}^{-1/2} \, {}^{\widetilde{\phi}}H_{uvu'v'}. \tag{ii}$$

There are four indices to account for the indices in $x$ and in $p$ in phase space for each of the two basis functions. Defining $M \equiv (m_{\max} + 1)$, the transformation of one matrix scales as $N^2\lceil M^2/2\rceil^2 = N^2\overline{M}$, where $N$ is the total number of basis functions. The prefactor $1/2^2$ stems from the symplicial truncation along the $m, n$ and $m', n'$ indices. The factor $(-1)^{n/2+mt+n'/2+m't'}$ prevents a sequential summation. Note that $N$ is independent of $M$. Even if a small basis is used, $\overline{M}$ can be significantly larger and is 3721 for $m_{\max} = 10$. This value may not be large enough if very high accuracies are needed, see the asymptotic behavior in Fig. i. However, in Ref. 1, a lower accuracy was sufficient and the authors used $m_{\max} = 6$ ($\overline{M} = 625$) to reach a relative error of $10^{-6}$. Further, a value of $m_{\max} = 4$ ($\overline{M} = 169$) has been used to give an accuracy of the eigenvalues within $\pm 0.02\,\mathrm{cm}^{-1}$, compared to $m_{\max} = 6$ for the $Ne_2$ potential.[1] One can do a further symplicial truncation of the sum requiring $|m| + |n| + |m'| + |n'| \leq m_{\max}$. Then, $\overline{M}$ would be 681 ($m_{\max} = 10$), 129 ($m_{\max} = 6$) or 41 ($m_{\max} = 4$). However, we found a decrease in accuracy from $\sim 10^{-10}$ to $10^{-7}$ including violation of the variational principle ($m_{\max} = 10$, error of the first eigenvalue in the harmonic oscillator) if this additional truncation is used. We found improved results by using the restriction $|m| + |n| + |m'| + |n'| \leq 1.5 \times m_{\max}$.

In the projected Weylet basis, the integral transformation is $\mathbf{W}^{\dagger}\mathbf{H}\mathbf{W}$, where $\mathbf{W}$ is given in Eq. (23) in the main article. This scales as $N^3$, independent of the required accuracy, because the definition of the projected Weylets is based on a finite basis whereas the Weylets are defined from an infinite-dimensional basis.

If a SoP form of the Hamiltonian is used, the transformation needs to be done only for matrices of one-dimensional bases. However, the number of sum terms of the Hamiltonian can be quite large and the $N^2\overline{M}$ scaling can become a bottleneck. For example, the number of terms required in a POTFIT expansion of a six-dimensional HONO potential energy surface is 3750 for a basis of with sizes $\{20, 20, 45, 35, 30, 35\}$ (without mode-combination).[4] A transformation of the POTFIT terms to the Weylet basis would require $3750 \times \overline{M} \times (2 \times 20^2 + 45^2 + 2 \times 35^2 + 30^2) = 8.6 \times 10^{10}$ summations. In the case of the projected Weylets, only $3750 \times (2 \times 20^3 + 45^3 + 2 \times 35^3 + 30^3) = 8.2 \times 10^8$ summations are needed — more than 100 times less than for the Weylets. For $m_{\max} = 6$ (4), the factor in saved summations is still 18 (4.7). Using the additional symplicial truncation, the factor would be 19 ($m_{\max} = 10$), 3.6 ($m_{\max} = 6$) or 1.2 ($m_{\max} = 4$). If $N > \overline{M}$, the Weylet transformation would be faster. However, a basis of this size is rarely needed, and at most in one or two dimensions. Further, the pW transformations can be readily implemented using BLAS calls. Due to the highly optimized matrix-matrix multiplication routines in BLAS implementations, an additional saving in computing time of $\sim 10\text{–}10^2$ (depending on the hardware) is possible. For very large basis sizes, one can also make use of sparse matrix-matrix multiplication.

## ii. Comparison between the Weylet basis and FGH

We compare a pruned Weylet basis for the simple harmonic oscillator,

$$\hat{H}_{\mathrm{HO}} = -\frac{1}{2}\frac{\mathrm{d}^2}{\mathrm{d}x^2} + \frac{1}{2}x^2 \tag{iii}$$

against the Fourier Grid Hamiltonian. There are many ways to prune a phase-space basis. Here, we use the simple energy-cutoff formula and restrict the Weylet basis by

$$|p_{\max}| = \sqrt{[E_{\mathrm{cut}} - V(x)]2m} \tag{iv}$$

and $E_{\mathrm{cut}} = 90$, $m = 1$. We further used a FGH which has the *same* basis size as the *pruned* Weylet basis and $x \in [-13.29, 13.29]$, which corresponds to the maximal $x$-range of the pruned Weylets. That is, the FGH describes a rectangle in phase space and the pruned Weylet basis an ellipse. The results are depicted in Table i. The FGH results are much more accurate, even though the basis size is not larger. Our pruned Weylet computation is in perfect agreement with a similar calculation of B. Poirier.[5] A pW computation based on the FGH-setup would yield the *same* eigenvalues as the FGH (up to rounding errors). However, the pW setup can be chosen to be identical to the pruned Weylets. Then, they exhibit almost the same eigenvalues as the pruned Weylets.

Table i: Comparison of the eigenenergies of the simple harmonic oscillator using a pruned Weylet basis and a Fourier Grid Hamiltonian that has the *same* size as the *pruned* Weylet basis, 92. For the pruned Weylet basis, an energy cutoff criterion of $E_{max} = 90$ has been chosen. Shown are the exact and numerical eigenenergies and the absolute error.

| E(exact) | E(pruned Weylet) | absolute error | E(FGH) | absolute error |
|---|---|---|---|---|
| 0.5 | 0.500 000 000 | $3.98 \times 10^{-10}$ | 0.500 000 000 | $8.10 \times 10^{-15}$ |
| 1.5 | 1.500 000 001 | $1.05 \times 10^{-9}$ | 1.500 000 000 | $3.77 \times 10^{-15}$ |
| 2.5 | 2.500 000 004 | $4.50 \times 10^{-9}$ | 2.500 000 000 | $1.02 \times 10^{-14}$ |
| 3.5 | 3.500 000 011 | $1.08 \times 10^{-8}$ | 3.500 000 000 | $4.44 \times 10^{-15}$ |
| 4.5 | 4.500 000 019 | $1.93 \times 10^{-8}$ | 4.500 000 000 | $-3.55 \times 10^{-15}$ |
| 5.5 | 5.500 000 030 | $3.02 \times 10^{-8}$ | 5.500 000 000 | $8.88 \times 10^{-15}$ |
| 6.5 | 6.500 000 043 | $4.31 \times 10^{-8}$ | 6.500 000 000 | $8.88 \times 10^{-15}$ |
| 7.5 | 7.500 000 057 | $5.65 \times 10^{-8}$ | 7.500 000 000 | $1.78 \times 10^{-15}$ |
| 8.5 | 8.500 000 073 | $7.26 \times 10^{-8}$ | 8.500 000 000 | $1.42 \times 10^{-14}$ |
| 9.5 | 9.500 000 093 | $9.33 \times 10^{-8}$ | 9.500 000 000 | $-7.11 \times 10^{-15}$ |
| 10.5 | 10.500 000 124 | $1.24 \times 10^{-7}$ | 10.500 000 000 | $-8.88 \times 10^{-15}$ |
| 11.5 | 11.500 000 176 | $1.76 \times 10^{-7}$ | 11.500 000 000 | $-1.60 \times 10^{-14}$ |
| 12.5 | 12.500 000 278 | $2.78 \times 10^{-7}$ | 12.500 000 000 | $-3.55 \times 10^{-15}$ |
| 13.5 | 13.500 000 483 | $4.83 \times 10^{-7}$ | 13.500 000 000 | $-7.11 \times 10^{-15}$ |
| 14.5 | 14.500 000 870 | $8.70 \times 10^{-7}$ | 14.500 000 000 | $-7.11 \times 10^{-15}$ |
| 15.5 | 15.500 001 520 | $1.52 \times 10^{-6}$ | 15.500 000 000 | $7.11 \times 10^{-15}$ |
| 16.5 | 16.500 002 496 | $2.50 \times 10^{-6}$ | 16.500 000 000 | $-2.84 \times 10^{-14}$ |
| 17.5 | 17.500 003 820 | $3.82 \times 10^{-6}$ | 17.500 000 000 | $-1.42 \times 10^{-14}$ |
| 18.5 | 18.500 005 484 | $5.48 \times 10^{-6}$ | 18.500 000 000 | $-7.11 \times 10^{-15}$ |
| 19.5 | 19.500 007 484 | $7.48 \times 10^{-6}$ | 19.500 000 000 | $-2.49 \times 10^{-14}$ |
| 20.5 | 20.500 009 834 | $9.83 \times 10^{-6}$ | 20.500 000 000 | $-1.07 \times 10^{-14}$ |
| 21.5 | 21.500 012 564 | $1.26 \times 10^{-5}$ | 21.500 000 000 | $-7.11 \times 10^{-15}$ |
| 22.5 | 22.500 015 680 | $1.57 \times 10^{-5}$ | 22.500 000 000 | $-1.78 \times 10^{-14}$ |
| 23.5 | 23.500 019 107 | $1.91 \times 10^{-5}$ | 23.500 000 000 | $-2.84 \times 10^{-14}$ |
| 24.5 | 24.500 022 633 | $2.26 \times 10^{-5}$ | 24.500 000 000 | $-1.42 \times 10^{-14}$ |
| 25.5 | 25.500 025 958 | $2.60 \times 10^{-5}$ | 25.500 000 000 | $-1.07 \times 10^{-14}$ |
| 26.5 | 26.500 028 840 | $2.88 \times 10^{-5}$ | 26.500 000 000 | $-1.78 \times 10^{-14}$ |
| 27.5 | 27.500 031 306 | $3.13 \times 10^{-5}$ | 27.500 000 000 | $-2.49 \times 10^{-14}$ |
| 28.5 | 28.500 033 920 | $3.39 \times 10^{-5}$ | 28.500 000 000 | $-1.78 \times 10^{-14}$ |
| 29.5 | 29.500 037 999 | $3.80 \times 10^{-5}$ | 29.500 000 000 | $-1.07 \times 10^{-14}$ |
| 30.5 | 30.500 045 676 | $4.57 \times 10^{-5}$ | 30.500 000 000 | $-4.62 \times 10^{-14}$ |
| 31.5 | 31.500 059 659 | $5.97 \times 10^{-5}$ | 31.500 000 000 | $1.88 \times 10^{-13}$ |
| 32.5 | 32.500 082 783 | $8.28 \times 10^{-5}$ | 32.500 000 000 | $-1.00 \times 10^{-12}$ |
| 33.5 | 33.500 117 681 | $1.18 \times 10^{-4}$ | 33.500 000 000 | $4.91 \times 10^{-12}$ |
| 34.5 | 34.500 166 917 | $1.67 \times 10^{-4}$ | 34.500 000 000 | $-2.35 \times 10^{-11}$ |
| 35.5 | 35.500 233 806 | $2.34 \times 10^{-4}$ | 35.500 000 000 | $1.05 \times 10^{-10}$ |
| 36.5 | 36.500 323 380 | $3.23 \times 10^{-4}$ | 36.500 000 000 | $-4.63 \times 10^{-10}$ |
| 37.5 | 37.500 442 936 | $4.43 \times 10^{-4}$ | 37.500 000 002 | $1.89 \times 10^{-9}$ |
| 38.5 | 38.500 602 055 | $6.02 \times 10^{-4}$ | 38.499 999 992 | $-7.63 \times 10^{-9}$ |
| 39.5 | 39.500 812 058 | $8.12 \times 10^{-4}$ | 39.500 000 028 | $2.84 \times 10^{-8}$ |
| 40.5 | 40.501 084 992 | $1.08 \times 10^{-3}$ | 40.499 999 894 | $-1.06 \times 10^{-7}$ |
| 41.5 | 41.501 435 088 | $1.44 \times 10^{-3}$ | 41.500 000 357 | $3.57 \times 10^{-7}$ |
| 42.5 | 42.501 871 271 | $1.87 \times 10^{-3}$ | 42.499 998 775 | $-1.22 \times 10^{-6}$ |

Further, we have compared both PvB, pW and the Weylets for the harmonic oscillator using different values of $E_{\text{cut}}$ resulting in different basis sizes. Fig. i shows the results. The error is evaluated by the Euclidian $L_2$ distance between the exact and the numerical energies. PvB is the most efficient scheme, followed by pW and the Weylets. Because of the same phase-space tiling, the errors of pW and the Weylets are very similar. Of course, these results cannot be generalized and it does not mean that, in general, PvB is more efficient than Weylets in the time-independent context.

The $\mathbf{S}^{-1/2}$ values for the creation of the Weylets have been taken from Ref. 2. There, they are listed up to 12 digits. Hence the asymptote of the Weylets which exhibit an error of $\sim 10^{-9}$ (accumulated for the first 42 eigenvalues) in the basis limit. In practice, this error does not matter.

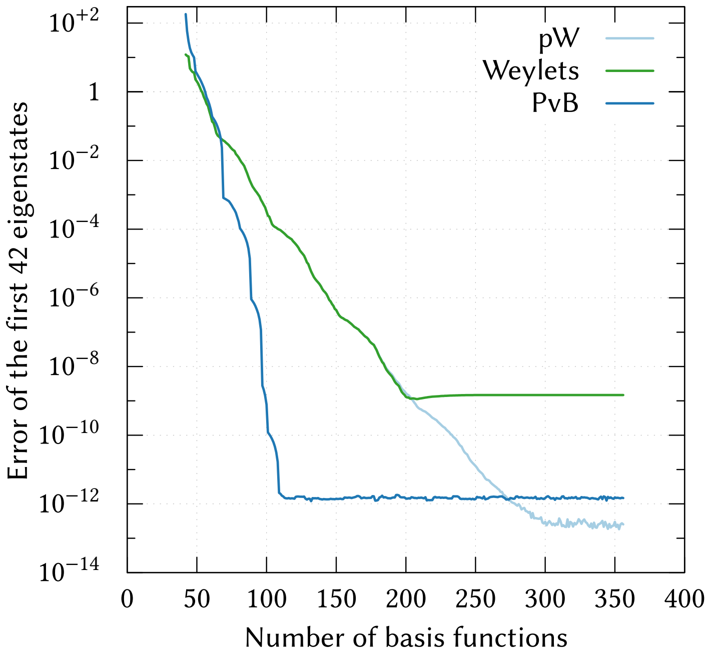


Figure i: Comparison of pruned pW, Weylets and PvB for the simple harmonic oscillator.

## iii. Phase-space representation of symmetric or asymmetric states

We represent the following two states

$$f_1(x) = \exp[-(x - 28.83)^2 + \mathrm{i} \times 14x] \times \frac{\exp(49)}{\pi}, \tag{v}$$

$$f_2(x) = \{\exp[-(x - 28.83)^2 + \mathrm{i} \times 14x] + \exp[-(x - 28.83)^2 - \mathrm{i} \times 14x]\} \times \frac{\exp(49)}{2\sqrt{\pi}} \tag{vi}$$

using PvB and pW. $|f_1\rangle$ is momentum-asymmetric whereas $|f_2\rangle$ is momentum-symmetric in phase-space. The phase-space-representation is shown in Fig. ii. Both states span roughly the same area in the pW representation whereas they span twice the area in PvB representation. With pW, the information about momentum-symmetry seems to be almost only described by the phase of the complex-valued coefficients. The needed area to describe the space is larger for pW than for PvB. This is also the case for a Weylet calculation. It seems that this is due to the inclusion of $\mathbf{S}^{-1/2}$ in the wavefunction expansion coefficients (compare with the discussion below Eq. (8) in the main article). If one uses the biorthogonal basis of the projected symmetrized Gaussians, the needed area is much more confined.

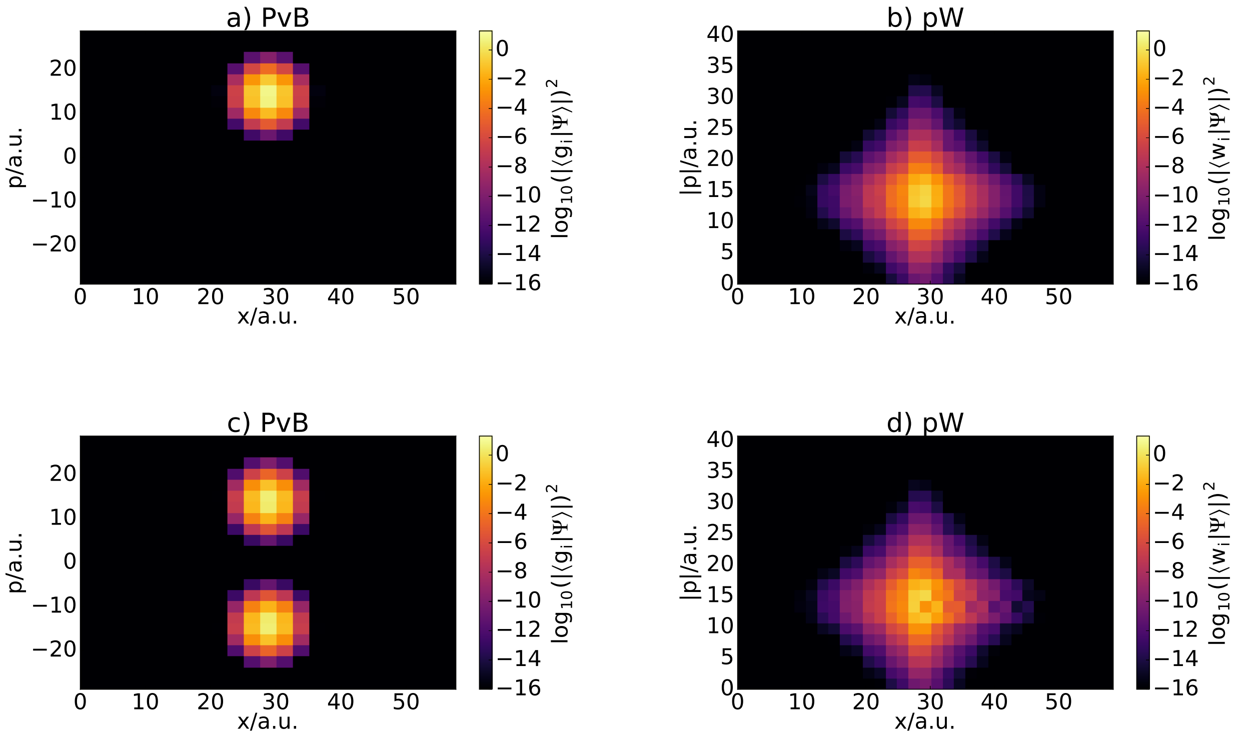


Figure ii: Phase-space-representation of the states $|f_1\rangle$, Eq. (v), in a) and b) and $|f_2\rangle$, Eq. (vi), in c) and d) using PvB and pW.

## References

[1] Lombardini, R.; Poirier, B. *J. Chem. Phys.* **2006**, *124*, 144107.

[2] Poirier, B.; Salam, A. *J. Chem. Phys.* **2004**, *121*, 1690.

[3] Poirier, B.; Salam, A. *J. Chem. Phys.* **2004**, *121*, 1704.

[4] Peláez, D.; Meyer, H.-D. *J. Chem. Phys.* **2013**, *138*, 014108.

[5] Poirier, B. private communication.
